# Supplementary material for: Safe Self-Refinement for Transformer-based Domain Adaptation
Source: arXiv:2204.07683 source file (2022-04-16)
Supplement: Supplementary file 1 [file Table_DomainNet_supp.latex]

\begin{tabular}{|p{0.9cm}<{\centering}|@{\hspace{0.05cm}}p{0.55cm}<{\centering}@{\hspace{0.05cm}}p{0.55cm}<{\centering}@{\hspace{0.05cm}}p{0.55cm}<{\centering}@{\hspace{0.05cm}}p{0.55cm}<{\centering}@{\hspace{0.05cm}}p{0.55cm}<{\centering}@{\hspace{0.05cm}}p{0.55cm}<{\centering}@{\hspace{0.2cm}}@{\hspace{0.0cm}}p{0.38cm}<{\centering}||p{0.9cm}<{\centering}|@{\hspace{0.05cm}}p{0.55cm}<{\centering}@{\hspace{0.05cm}}p{0.55cm}<{\centering}@{\hspace{0.05cm}}p{0.55cm}<{\centering}@{\hspace{0.05cm}}p{0.55cm}<{\centering}@{\hspace{0.05cm}}p{0.55cm}<{\centering}@{\hspace{0.05cm}}p{0.55cm}<{\centering}@{\hspace{0.2cm}}@{\hspace{0.0cm}}p{0.38cm}<{\centering}||p{0.9cm}<{\centering}|@{\hspace{0.05cm}}p{0.55cm}<{\centering}@{\hspace{0.05cm}}p{0.55cm}<{\centering}@{\hspace{0.05cm}}p{0.55cm}<{\centering}@{\hspace{0.05cm}}p{0.55cm}<{\centering}@{\hspace{0.05cm}}p{0.55cm}<{\centering}@{\hspace{0.05cm}}p{0.55cm}<{\centering}@{\hspace{0.2cm}}@{\hspace{0.0cm}}p{0.38cm}<{\centering}|}
\hline  \textbf{\tabincell{c}{CD-\\Trans\cite{xu2021cdtrans}}}  & clp & inf & pnt & qdr & rel & skt & Avg. &  \textbf{ViT}  & clp & inf & pnt & qdr & rel & skt & Avg. &  \textbf{Baseline}  & clp & inf & pnt & qdr & rel & skt & Avg.  \\\hline clp & -  &  27.5 &  57.4 &  22.3 &  76.2 &  57.3 & 48.1 & clp & -  &  27.2 &  53.1 &  13.2 &  71.2 &  53.3 & 43.6 & clp & -  &  30.9 &  53.3 &  16.3 &  72.7 &  55.4 & 45.7  \\inf &  60.2 & -  &  52.4 &  11.5 &  74.8 &  48.9 & 49.6 & inf &  51.4 & -  &  49.3 &  4.0 &  66.3 &  41.1 & 42.4 & inf &  43.0 & -  &  40.8 &  7.8 &  56.4 &  35.9 & 36.8  \\pnt &  62.1 &  25.6 & -  &  10.5 &  73.9 &  49.6 & 44.3 & pnt &  53.1 &  25.6 & -  &  4.8 &  70.0 &  41.8 & 39.1 & pnt &  55.7 &  28.6 & -  &  7.4 &  70.5 &  48.3 & 42.1  \\qdr &  3.5 &  0.5 &  0.6 & -  &  2.6 &  6.0 & 2.6 & qdr &  30.5 &  4.5 &  16.0 & -  &  27.0 &  19.3 & 19.5 & qdr &  25.5 &  5.2 &  9.7 & -  &  15.5 &  17.1 & 14.6  \\rel &  49.0 &  20.2 &  47.9 &  9.0 & -  &  33.5 & 31.9 & rel &  58.4 &  29.0 &  60.0 &  6.0 & -  &  45.8 & 39.9 & rel &  62.3 &  32.5 &  62.5 &  8.2 & -  &  50.7 & 43.2  \\skt &  68.3 &  21.7 &  49.1 &  17.8 &  72.8 & -  & 45.9 & skt &  63.9 &  23.8 &  52.3 &  14.4 &  67.4 & -  & 44.4 & skt &  66.4 &  30.6 &  58.0 &  18.1 &  70.1 & -  & 48.6  \\Avg. & 48.6 & 19.1 & 41.5 & 14.2 & 60.1 & 39.1 & \cellcolor{tbgray}37.1 & Avg. & 51.5 & 22.0 & 46.1 & 8.5 & 60.4 & 40.3 & \cellcolor{tbgray}38.1 & Avg. & 50.6 & 25.6 & 44.9 & 11.6 & 57.0 & 41.5 & \cellcolor{tbgray}38.5\\ \hline \hline  \textbf{VAT\cite{miyato2018virtual}}  & clp & inf & pnt & qdr & rel & skt & Avg. &  \textbf{\tabincell{c}{SSRT\\\ raw input}}  & clp & inf & pnt & qdr & rel & skt & Avg. &  \textbf{\tabincell{c}{SSRT\\\{0\}}}  & clp & inf & pnt & qdr & rel & skt & Avg.  \\\hline clp & -  &  33.1 &  57.1 &  19.5 &  75.8 &  59.8 & 49.0 & clp & -  &  32.7 &  60.0 &  19.0 &  75.3 &  59.8 & 49.3 & clp & -  &  33.2 &  59.7 &  19.6 &  75.3 &  58.7 & 49.3  \\inf &  48.3 & -  &  45.2 &  9.8 &  55.0 &  37.4 & 39.2 & inf &  55.0 & -  &  54.0 &  8.9 &  67.8 &  48.1 & 46.8 & inf &  54.8 & -  &  53.5 &  9.3 &  67.7 &  46.1 & 46.3  \\pnt &  60.0 &  30.9 & -  &  7.9 &  71.1 &  52.6 & 44.5 & pnt &  61.6 &  28.6 & -  &  8.2 &  71.3 &  55.4 & 45.0 & pnt &  61.2 &  29.0 & -  &  7.1 &  71.2 &  55.0 & 44.7  \\qdr &  26.7 &  5.4 &  9.2 & -  &  18.1 &  18.3 & 15.5 & qdr &  36.3 &  6.2 &  16.1 & -  &  32.1 &  31.2 & 24.4 & qdr &  40.8 &  7.0 &  13.2 & -  &  35.4 &  31.1 & 25.5  \\rel &  68.7 &  35.3 &  65.0 &  7.8 & -  &  56.8 & 46.7 & rel &  69.8 &  35.6 &  66.1 &  12.4 & -  &  59.2 & 48.6 & rel &  69.6 &  35.7 &  65.7 &  10.7 & -  &  58.7 & 48.1  \\skt &  70.2 &  33.3 &  65.0 &  17.6 &  72.2 & -  & 51.7 & skt &  70.3 &  30.5 &  62.3 &  20.0 &  73.2 & -  & 51.3 & skt &  69.7 &  32.1 &  62.0 &  19.0 &  72.8 & -  & 51.1  \\Avg. & 54.8 & 27.6 & 48.3 & 12.5 & 58.4 & 45.0 & \cellcolor{tbgray}41.1 & Avg. & 58.6 & 26.7 & 51.7 & 13.7 & 63.9 & 50.8 & \cellcolor{tbgray}44.2 & Avg. & 59.2 & 27.4 & 50.8 & 13.1 & 64.5 & 49.9 & \cellcolor{tbgray}44.2\\ \hline \hline  \textbf{\tabincell{c}{SSRT\\\{4\}}}  & clp & inf & pnt & qdr & rel & skt & Avg. &  \textbf{\tabincell{c}{SSRT\\\{8\}}}  & clp & inf & pnt & qdr & rel & skt & Avg. &  \textbf{\tabincell{c}{SSRT\\\{0,4,8\}}}  & clp & inf & pnt & qdr & rel & skt & Avg.  \\\hline clp & -  &  31.8 &  58.9 &  17.8 &  75.7 &  59.4 & 48.7 & clp & -  &  32.4 &  59.0 &  18.6 &  75.6 &  59.9 & 49.1 & clp & -  &  33.8 &  60.2 &  19.4 &  75.8 &  59.8 & 49.8  \\inf &  53.5 & -  &  50.5 &  8.6 &  67.8 &  47.5 & 45.6 & inf &  55.9 & -  &  54.8 &  7.6 &  68.5 &  48.2 & 47.0 & inf &  55.5 & -  &  54.0 &  9.0 &  68.2 &  44.7 & 46.3  \\pnt &  61.3 &  29.2 & -  &  8.1 &  71.3 &  54.3 & 44.8 & pnt &  61.5 &  27.4 & -  &  8.5 &  71.4 &  54.6 & 44.7 & pnt &  61.7 &  28.5 & -  &  8.4 &  71.4 &  55.2 & 45.0  \\qdr &  42.5 &  7.7 &  17.0 & -  &  23.3 &  33.4 & 24.8 & qdr &  33.6 &  5.7 &  11.3 & -  &  31.4 &  31.8 & 22.7 & qdr &  42.5 &  8.8 &  24.2 & -  &  37.6 &  33.6 & 29.3  \\rel &  68.7 &  36.1 &  65.5 &  8.2 & -  &  57.6 & 47.2 & rel &  69.6 &  36.2 &  65.9 &  6.9 & -  &  58.1 & 47.3 & rel &  69.9 &  37.1 &  66.0 &  10.1 & -  &  58.9 & 48.4  \\skt &  70.1 &  31.8 &  62.2 &  17.7 &  73.1 & -  & 51.0 & skt &  69.9 &  30.9 &  62.3 &  19.8 &  73.3 & -  & 51.2 & skt &  70.6 &  32.8 &  62.2 &  21.7 &  73.2 & -  & 52.1  \\Avg. & 59.2 & 27.3 & 50.8 & 12.1 & 62.2 & 50.4 & \cellcolor{tbgray}43.7 & Avg. & 58.1 & 26.5 & 50.6 & 12.3 & 64.0 & 50.5 & \cellcolor{tbgray}43.7 & Avg. & 60.0 & 28.2 & 53.3 & 13.7 & 65.3 & 50.4 & \cellcolor{tbgray}\HL{45.2}\\ \hline 
\end{tabular}
